# Supplementary material for: Delving into the Continuous Domain Adaptation
Source: arXiv:2208.13121 source file (2022-08-28)
Supplement: Supplementary file 1 [file analysis.tex]

\section{Analysis and Discussion}

\subsection{Motivation Clarifications}

We clarify and re-emphasize essential motivations of the new CDA task and the proposed method. 

\textbf{Motivation of the CDA Formulation.} The novel CDA problem is analogous to practical setting where we are given a dataset in the real-world application with a continuously varying attribute. Furthermore, such attribute variations, although sometimes tiny, will destroy the model developed using partially annotated data obtained from the dataset. In the CDA task, all domains are sampled based on the continuous attribute and the domain variations are mainly caused by the attribute variations. The task is practical as we are only given two source domains with data and annotations and the un-annotated probe target domain data, with the goal of learning a generalized model using these information. Note that the test data also comprises unseen domains. 

\textbf{Motivation of the Alternating Direction Training Strategy.} The main objective of CDA is to learn a generalized model tackling discrepancies among all domains sampled on a continuous attribute. To handle the statistics of unseen domain data, our strategy is to study the geometry of the continuous attribute and use it as an inductive bias in the modelling. Inspired by this principle, we design the alternating direction training strategy, including two steps: Pull and Shrinkage. In P step, we regard the trajectory formed by the two source domains as the inductive bias and pull target domains to the trajectory so that unseen target domains have higher chance to be close to the trajectory as well. In S step, we progressively shrink and shorten the trajectory. Alternating the two steps in the training, the proposed method is proved to be able to generalize to unseen target domains. 

% \begin{figure}[!t]
% \centering
% \includegraphics[width=\columnwidth]{figure/early.pdf}
% \caption{(a)Source-target discrepancy.(b)Source-source discrepancy. Red circles denote the biased discrepancies during early training.}
% \label{ana}
% \end{figure}

\textbf{The definitions of the auxiliary classifier $F'$ and the discrepancy measure.} $F'$ and $F$ are both classifiers with the same architecture and take the same input and outputs. Note that content classifiers $F$ and $F_2$ are used to classify content labels in each source domain, while auxiliary classifiers $F_1'$ and $F_2'$ are used to estimate the discrepancies (together with content classifiers). $p'(\hat{y}|e)$ indicates the probabilities of that $F'$ and $F$ predicting the same class. The discrepancy between $P$,$Q$ is formally defined as: 
\begin{align}
\mathcal{D}(e_P,e_Q) = \sup_{F'}\mathbb{E}_P\log p'(\hat{y}|e) + \mathbb{E}_Q \log(1-p'(\hat{y}|e)).
\end{align}
% \begin{align}
% \mathcal{D}(e_P,e_Q) = \sup_{F'}\mathbb{E}_P\log p'(\hat(y)|e) + \mathbb{E}_Q \log(1-p'(\hat(y)|e)).
% \end{align}
It can be derived into the form of JS divergence(see section 3.3).

%  It can be observed that some methods localize different class-specific image regions in domains. For example, in CIDA, model pays more attention on eyes in two source domains, while in localize forehead in some unseen target domains which leads to misclassification. As for our method(the last row), model shows the same localization, eye, in all domains, and achieve right classifications. The results show that our method can localize the discriminative image regions without the impact of domain shift.  
\subsection{Analysis of the Method Effectiveness}
\textbf{T-SNE Results} In Figure \ref{mis-tsne}, we visualize the T-SNE feature of target, source domains among different training epochs. It can be observed that the source domain features (blue and orange) points are gradually spreading to the grey zone (all target domains). Finally when it comes to epoch 150, and 200, the T-SNE converges. 

\textbf{Detailed Sub-Domain Accuracy} As shown in Table \ref{ana_err}, the sub-domain accuracy is reported in the continuous DA task. It can be observed that our method can not only outperform other methods in unseen target domains (U), probe target domains (P) but also can outperform the source-only model on source domains (S1,S2). It is a very essential observations as it proves that our training strategy works as a specially designed augmentation procedure and helps generalization. 

As it outperforms the supervised learning method on the source domains, it proves that our method won't "forget" the knowledge from the source domain and regard the overall performances in all the continuous domains as the training objective. 

\textbf{Failure Cases} In addition, we present some hard samples and failure cases that are misclassified by all methods in Figure \ref{mis-hard}. We hypothesize that this is mainly due to the poor quality of GAN in the synthesis procedure. The genuine cases of this observation is worth investigations in the future.

\input{tables/acc_ana}

% \subsection{Insights}

% In addition, we present some hard samples that are misclassified by all methods in Figure \ref{mis}.
% \input{tables/acc_ana}

% - when budgets are limited, how to select the best domains to annotate. 

\begin{figure}[t]
\centering
\includegraphics[width=0.9\columnwidth]{figure/hard_sample.pdf} 
\caption{Examples that are misclassified by all methods.}.
\label{mis-hard}
\end{figure}

\begin{figure}[t]
\centering
\includegraphics[width=0.9\columnwidth]{figure/5_tsne.pdf} 
\caption{Visualization of t-SNE in different epochs.}.
\label{mis-tsne}
\end{figure}

\subsection{Theoretical Justifications}
\textbf{Optimization in P step} We first consider the optimization problem we have defined in stage P:
\begin{align}
 \mathcal{D}_{1}(e_{s_1},e_{t_i}) + \mathcal{D}_{2}(e_{s_2},e_{t_i}) \label{dss}\\
 =\sum_{j=1,2}\max_{F_j'}\big[-\mathbb{E}_{e_{s_1}\sim P_{s_j}}\log[\sigma_{h_{F_j}(e)}\circ F'_j(e)]  \notag  \\
 - \mathbb{E}_{e_{t_i}\sim P_{t_i}}\log[1-\sigma_{h_{F_j}(e)} \circ F'_j(e)]\big] \label{eq3}  \notag \\
\end{align}
Let $J_j(e) = \sigma_{h_{F_j}(e)}\circ F'_j(e)$, then,
\begin{align}
&\mathcal{D}_{1}(e_{s_1},e_{t_i}) + \mathcal{D}_{2}(e_{s_2},e_{t_i})  \notag \\
 = &\max_{F_1'} \int_{e}-P_{s_1} \log J_1(e) - {P_{t_i}}\log(1- J_1(e)) de \notag \\
  +&\max_{F_2'} \int_{x} - P_{s_2} \log J_2(e)  - {P_{t_i}}\log(1-J_2(e) ) de
\end{align}
Eq.(3) reaches the largest when
\begin{align}
\label{op1}
 J_1(e) = \sigma_{h_{F_1}(e)}\circ F'_1(e) = \frac{ P_{s_1}}{P_{s_1} + P_{t_i}}\\
 \label{op2}
 J_2(e) = \sigma_{h_{F_2}(e)}\circ F'_2(e) = \frac{ P_{s_2}}{P_{s_2} + P_{t_i}}.
\end{align}
Replace Eq.\eqref{op1} and Eq.\eqref{op2} into Eq.\eqref{dss},
% If we substitute Eq \eqref{op1} into Eq \eqref{alpha1}, the target-source discrepancy is equivalent to a JS-divergence:
% \begin{align}
% \label{js1}
% D_{s,t}(T,S) = \text{JS}(P_{s1}||P_t) + \text{JS}(P_{s2}||P_t) - 4\log{2}
% \end{align}
\begin{align}
&\mathcal{D}_{1}(e_{s_1},e_{t_i}) + \mathcal{D}_{2}(e_{s_2},e_{t_i})  \notag \\
=& \max_{F_1'} \int_{e}-P_{s_1} \log \frac{ P_{s_1}}{P_{s_1} + P_{t_i}} - {P_{t_i}}\log\frac{ P_{t_i}}{P_{s_1} + P_{t_i}} de \notag \\
  + &\max_{F_2'} \int_{x} - P_{s2} \log \frac{ P_{s_2}}{P_{s_2} + P_{t_i}}  - {P_{t_i}}\log\frac{ P_{t_i}}{P_{s_s} + P_{t_i}} de\notag \\
=& JS(P_{s_1}||P_{t_i}) + JS(P_{s_2}||P_{t_i}) + 2\log2
\end{align}
Thus,
\begin{align}
&\min_{E} \mathcal{D}_{1}(e_{s_1},e_{t_i}) + \mathcal{D}_{2}(e_{s_2},e_{t_i})  \notag \\
=& \min_{E} JS(P_{s_1}||P_{t_i}) + JS(P_{s_2}||P_{t_i}) + 2\log2 \notag \\
=& \min_{E} JS(P_{s_1}||P_{t_i}) + JS(P_{s_2}||P_{t_i})
\end{align}
\textbf{Optimization in S step} The optimization problem is defined as follow:
\begin{align}
&\mathcal{D}_{1}(e_{s_1},e_{s_2}) + \mathcal{D}_{2}(e_{s_2},e_{s_1})  \label{dsst} \\
 = &\max_{F_1'} \int_{e}-P_{s_1} \log J_1(e) - {P_{s_1}}\log(1- J_1(e)) de \notag \\
  +&\max_{F_2'} \int_{x} - P_{s_2} \log J_2(e)  - {P_{s_1}}\log(1-J_2(e) ) de
\end{align}
Eq.(9) reaches the largest when
\begin{align}
\label{op11}
 J_1(e) = \sigma_{h_{F_1}(e)}\circ F'_1(e) = \frac{ P_{s_1}}{P_{s_1} + P_{s_2}}\\
 \label{op22}
 J_2(e) = \sigma_{h_{F_2}(e)}\circ F'_2(e) = \frac{ P_{s_2}}{P_{s_1} + P_{t_2}}.
\end{align}
Replace Eq.\eqref{op11} and Eq.\eqref{op22} into Eq.\eqref{dsst},
\begin{align}
&\mathcal{D}_{1}(e_{s_1},e_{s_2}) + \mathcal{D}_{2}(e_{s_2},e_{s_1})\\
=&2JS(P_{s_1}||P_{S_2}) + 4\log2
\end{align}
Thus,
\begin{align}
&\min_{E} \mathcal{D}_{1}(e_{s_1},e_{s_2}) + \mathcal{D}_{2}(e_{s_2},e_{s_1})  \notag \\
=& \min_{E} 2JS(P_{s_1}||P_{s_2}) + 4\log2 \notag \\
=& \min_{E} JS(P_{s_1}||P_{s_2}) \end{align}

\textbf{Global optimum.} Eq.(8) has the minimum at $P_{s_1}=P_{t_i}$ or $P_{s_2}=P_{t_1}$, while Eq.(15) at $P_{s_1}=P_{s_2}$. Thus, two stages has the global optimum at $P_{t}=P_{s_1}=P_{s_1}$.
