# Supplementary material for: Delving into the Continuous Domain Adaptation
Source: arXiv:2208.13121 source file (2022-08-28)
Supplement: Supplementary file 2 [file result.tex]

\section{Additional Results}
% To demonstrate our method's universality, we further evaluate on five classic digits datasets \chensays{give a figure here.} (MNIST\cite{lecun1998gradient},USPS\cite{hull1994database}, MNIST-M\cite{ganin2015unsupervised},SynNum\cite{ganin2015unsupervised}, and SVHN\cite{netzer2011reading}). MNIST and USPS are datasets for handwritten digits, while MNIST-M and SynNum are for syntheic numbers. SVHN are collected form street view housing numbers.  All images are resized to $32 \times 32$ and 3 channels. Besides, no further transforms is applied to the data. We designate each dataset as a domain. As there is not a explicit attribute among them, we sort them by the complexity: MNIST, USPS,  SynNum, MNIST-M, SVHN. For each domain, we follow the origin training/testing split. Beacuse of the limited number of domains, we adopt different splits: MNIST and SHVN are used as source domain, and one of the rest three is used as probe target domain. Besides, we record the accuracy of each domain, as the number of samples are unbalance in different domains.

\subsection{More comparison methods}
We compare with other methods, including source-only model with a Maximum Mean Discrepancy (MMD) discrepancy measurement. In addition, we compare with the state-of-the-art Domain Generalization (DG) method, and continual learning method.
\begin{table*}[t]
\small
\caption{Comparision Results (\%) in SmallNorb Dataset.}
\centering
% \resizebox{\linewidth}{!}{
\begin{tabular}{c|c|cccc|cccc|cccc|c}
\hline
\multirow{2}{*}{Method}&  P 1& \multicolumn{4}{c|}{P 2} & \multicolumn{4}{c|}{P 3} & \multicolumn{4}{c|}{P 4}& \multirow{2}{*}{Avg.}\\
   & S 1&S 1   &S 2     &S 3     &S 4    &S 1     &S 2     &S 3     &S 4    &S 1     &S 2     &S 3     &S 4  \\
\hline
So &85.1 &88.8 &88.8 &88.8 &88.8 & 86.8 &86.8 &86.8 &86.8 &86.5&86.5&86.5&86.5&87.1\\
So + MMD &78.2 &80.6&82.5 &79.4 &77.4 &80.2 &80.3 &73.8 &72.8 &80.7 &80.1 &78.5&77.0&78.6\\
So + MixStyle &84.0&88.0&88.0&88.0&88.0 &87.1 &87.1 &87.1 &87.1 &87.1 &87.1 &87.1 &87.1&87.1\\
CUA &84.8 & 86.8 &86.4 &83.9 &85.8 &85.5 &87.5 &84.8 &87.4 &82.8 &83.0 &81.0 &85.9 &85.0\\
EDA &45.3 &41.7 &49.0 &65.9 &66.0 &38.1  &42.1 &55.3 &51.8 &39.6 &43.4 &69.9 &65.1 &51.6\\
\hline  
Ours & \textbf{91.5}& \textbf{90.5}& \textbf{ 90.3}&     \textbf{89.6}&    \textbf{89.8}&  \textbf{87.6}&    \textbf{89.5}&     \textbf{87.4}&    \textbf{89.7}&   \textbf{87.8} &    \textbf{89.4}&     \textbf{87.8} &\textbf{90.1} & \textbf{89.3}\\
\hline 
\end{tabular}
% }

\label{sonorb}
\end{table*}

\textbf{Compare with Single-Domain DA modules.}
MMD \cite{tolstikhin2016minimax} is a popular discrepancy measurement in UDA. We adopt to compare with the method using MMD on the source only model to reduce the cross-domain discrepancy. The results are shown in Table \ref{sonorb}, denoted as So+MMD. We can observe that So+MMD leads to degraded performances. We conjecture that MMD failed to measure the discrepancy among source domain and unseen target domains, therefore disturbing the geometry of continuous domains. Consequently, the discrepancy among unseen target domains are enlarged.

\textbf{Compare with DG method.}
Due to similarities to DG methods, we also reproduce the MixStyle \cite{zhou2021mixstyle}, the SOTA DG method which mixes instance-level feature to perform DG. We add the MixStyle module after the third convolution layer of source-only model to mix features from two source domains. The results are shown in Table \ref{sonorb}, denoted as So+MixStyle. It seems that the performances are very close to the So performances. It demonstrates the complexity of the geometry of continuous domain and because of this, the mixture of two source domains cannot approximate the target domains accurately.

\textbf{Compare with Continual learning method.}
We reproduce the continual learning method on the CDA datasets, including Continuous Unsupervised Adaptation(CUA)\cite{bobu2018adapting}, and Evolving domain adaptation(EDA)\cite{NEURIPS2020_fd69dbe2}. The results are shown in Table \ref{sonorb}. It seems that continual learning leads to degraded performances. We conjecture that these methods fail to general on the whole distribution because of ignoring the unseen domains.

\subsection{More results of ablation study on CDA}
We perform ablation studies on all splits in Small Norb dataset to support the main submission ablation studies. The results are shown in Table \ref{analy}. It verifies the effectiveness of each proposed main contribution, including: 1) the discrepancy measure, 2) the alternating two-stage training strategy, 3) the continuity constraint using gradient plenty, and 4) feature queues. 

\subsection{Evaluation on Existing Multi-Domain Benchmark}
\begin{figure}[t]
\centering
\includegraphics[width=0.9\columnwidth]{figure/digits.pdf} 
\caption{Examples of C-DIGIT benchmark.}.
\label{dig}
\end{figure}
To demonstrate the effectiveness of our method in other multi-domain adaptation tasks (without continuous attribute variations observed), we evaluate it using the C-DIGIT \cite{compounddomainadaptation} benchmark including five classic digits datasets (as shown in Figure \ref{dig}): MNIST(mt)\cite{lecun1998gradient}, USPS(up)\cite{hull1994database}, MNIST-M(mm)\cite{ganin2015unsupervised}, SynNum(sy)\cite{ganin2015unsupervised}, and SVHN(sv)\cite{netzer2011reading}. Note that although the C-DIGIT dataset is not able to evaluate the continuous DA method, we can use it to evaluate our method handling multiple domain discrepancies caused by discrete and irrelevant domain attribute variations. All images are resized to $32 \times 32$ and 3 channels and no further transforms are applied to the data. We regard each dataset of the five digit ones as a single domain. As the domain attribute and the variations cannot be explicitly observed among these datasets, we sort them by the complexity, assuming that they lie on the continuous attribute space in the following order: MNIST, USPS,  SynNum, MNIST-M, SVHN. Due to the limited domain numbers, we evaluate our method using the following setup: MNIST and SHVN are used as source domain, and one of the rest three is used as probe target domain and the rest target domain is regarded as the unseen test ones. 
% Besides, we report the accuracy of each domain, as the number of samples are unbalance in different domains.

The results are shown in Table \ref{ana_digits}. It seems that the proposed method is able to outperform other comparison methods and can reduce multi-domain discrepancies caused by discrete and irrelevant domain attribute variations. Moreover, we evaluated our method for multi-source and multi-target DA in Table \ref{mtda}. It shows that our method is effective in multi-target DA setting. 

\subsection{Commonality and uniqueness. } From the mentioned comparison and the main submission, we can observe that a few single-domain, multi-source/target DA and DG methods, as well as continual learning method, are applicable to CDA, but achieve worse performances than ours. It shows the \textbf{\textit{uniqueness}} of CDA. In addition, our method is applicable to Multi-Source and Multi-Target DA, achieving SOTA results.  It demonstrates the \textbf{\textit{commonality}} of CDA.

% To demonstrate our method's universality, we further evaluate on five classic digits datasets (as shown in Figure \ref{dig}): \chensays{give a figure here.} MNIST(mt)\cite{lecun1998gradient},USPS(up)\cite{hull1994database}, MNIST-M(mm)\cite{ganin2015unsupervised},SynNum(sy)\cite{ganin2015unsupervised}, and SVHN(sv)\cite{netzer2011reading}. MNIST and USPS are datasets for handwritten digits, while MNIST-M and SynNum are for syntheic numbers. SVHN are collected form street view housing numbers.  All images are resized to $32 \times 32$ and 3 channels. Besides, no further transforms is applied to the data. We designate each dataset as a domain. As there is not a explicit attribute among them, we sort them by the complexity: MNIST, USPS,  SynNum, MNIST-M, SVHN. For each domain, we follow the origin training/testing split. Beacuse of the limited number of domains, we adopt different splits: MNIST and SHVN are used as source domain, and one of the rest three is used as probe target domain. Besides, we record the accuracy of each domain, as the number of samples are unbalance in different domains.
\begin{table*}[t]
\small
% \vspace{-3mm}
\centering
\caption{Analysis Results (\%) in Small Norb Dataset.}
% \fontsize{7.7}{8.5}\selectfont
% \setlength\tabcolsep{0.55pt}
\begin{tabular}{lrrrrrrrrrrrrrr}
\hline 
\multirow{2}{*}{Method}&  P 1& \multicolumn{4}{c}{P 2} & \multicolumn{4}{c}{P 3} & \multicolumn{4}{c}{P 4}& \multirow{2}{*}{Avg.}\\
   & S 1&S 1   &S 2     &S 3     &S 4    &S 1     &S 2     &S 3     &S 4    &S 1     &S 2     &S 3     &S 4  \\
\hline  
 Variant 1 &  88.6&  87.2&     87.1&     87.4&    88.8&  88.2&    87.3&     86.4&    86.4&   87.7&    86.5& 86.4& 87.3& 87.3 \\
 Variant 2 &  83.4&    87.6&     87.5&     86.4&    87.1&  84.0&    84.2&     85.5&    86.8&   83.5&    85.6&     85.6& 87.1&85.7\\
 Variant 3 &  88.1&    86.6&     88.4&     88.0&    87.3&  88.3&    87.4&     85.7&    87.5&   86.5&    88.2&     86.6& 87.6 &87.4\\
 Variant 4 &  86.4&    86.7&     88.5&     86.0&    87.2&  85.2&    86.6&     85.8&    87.8&   85.1&    86.7&     85.6& 87.0 &86.5\\
 Variant 5 &  83.4&    85.1&     85.4&     82.5&   87.0 &  85.9&    87.5&     84.5&    86.4&   86.5&    87.3&     84.5& 86.5&85.6\\
 Variant 6 &  90.2&    86.5&     89.7&     88.9&   89.0 &  87.5&    89.3&     87.4&    89.1&   88.7&    89.1&     87.5 & 89.3&88.6\\
 Variant 7 &  89.8&    89.1&     89.1&    88.3&  88.0 &  89.1&    89.1&     88.8&    88.1&   87.9&    87.9&     85.9&  87.6& 88.4\\
\hline  
Ours & \textbf{91.5}&    \textbf{90.5}&  \textbf{90.3}&     \textbf{89.6}&    \textbf{89.8}&  \textbf{87.6}&    \textbf{89.5}&     \textbf{87.4}&    \textbf{89.7}&   \textbf{87.8}&    \textbf{89.4}&     \textbf{87.8}& \textbf{90.1}& \textbf{89.3}\\
\hline
\end{tabular}

\label{analy}
\end{table*}
\begin{table}[t]
\centering
\caption{Comparision Results (\%) in five digits datasets.mm and sv are source domains and we test on mm.}
\begin{tabular}{c|c|c}
\hline
\multirow{2}{*}{Method} &\multicolumn{2}{c}{probe target domain}\\
&up & sy \\
\hline
SO &45.4 &45.4\\
CIDA &43.9 &48.6 \\
ATDOC &40.6 &50.1  \\
BCDM &27.6 &40.2\\
\hline 
Ours &\textbf{49.5} &\textbf{53.3}\\
\hline 
\end{tabular}

\label{ana_digits}
\end{table}

% \begin{table*}[t]
% \small
% \caption{Comparision Results (\%) in five digits datasets.\chensays{@yinsong, please change this in priority.}}
% \centering
% \begin{tabular}{c|c|c|c|c}
% \hline 
% Src. Domain& \multicolumn{2}{c|}{up} & \multicolumn{2}{c|}{sy} \\
% \hline 
% mt, sv& mt& up& sy& mm&  sv&  mt& up& sy& mm&  sv&  mt& up& sy& mm&  sv  \\
% \hline  
% SO &99.2&96.7&86.5&45.4&90.3 &99.2&96.1&89.5&45.4&90.3&99.2&96.1&86.5&45.4&90.3\\
% CIDA &93.8&80.6&70.1&43.9&71.5&98.2&92.5&78.9&48.6&84.8 &98.8&93.7&85.9&53.6&88.8\\
% ATDOC &98.3&95.4&73.1&40.6&80.7 &98.9&92.7&83.4&50.1&86.9  &98.1&92.7&75.6&45.2&82.3\\
% BCDM &91.3&25.2&48.5&27.6&68.2 &96.1&88.2&88.3&40.2&82.0&97.4&90.8&89.1&40.7&83.1\\
% DRT &99.1&96.1&83.9&47.7&88.9 &98.7&93.2&79.8&47.19&85.6 &99.1&95.6&84.3&48.9&88.9\\
% \hline  
% Ours &96.2&92.5&72.9&49.5&72.7 &94.3&83.5&76.4&53.3&73.5&89.3&80.6&71.1&55.9&69.6\\
% \hline 
% \end{tabular}
% \label{ana_digits}
% \end{table*}

\begin{table}[h]
\centering
\caption{Multi-target DA results (\%) in Digit-Five.}
\small
\begin{tabular}{c|c|c|c|c}
\hline
%'mnist', 'usps',  'syn', 'mnist_m', 'svhn'
%mt, up, sv, sy, mm are abbreviations for MNIST, USPS, SVHN, Synthetic Digits, MNIST-M
Dataset &mt & mm & sv& up \\
& $\rightarrow$up, sy& $\rightarrow$mt,up& $\rightarrow$mt,mm&$\rightarrow$sy,mm\\
\hline
SO & 30.9 &92.0 &51.3 &23.0\\
Ours &34.9 &93.4 &73.0 &41.9\\
\hline
\end{tabular}

\label{mtda}
\end{table}
