# Supplementary material for: Delving into the Continuous Domain Adaptation
Source: arXiv:2208.13121 source file (2022-08-28)
Supplement: Supplementary file 3 [file abla.tex]

\begin{table*}[t]
\small
% \vspace{-3mm}
\centering
\caption{Analysis Results (\%) in Small Norb Dataset.}
% \fontsize{7.7}{8.5}\selectfont
% \setlength\tabcolsep{0.55pt}
\begin{tabular}{lrrrrrrrrrrrrrr}
\hline 
\multirow{2}{*}{Method}&  P 1& \multicolumn{4}{c}{P 2} & \multicolumn{4}{c}{P 3} & \multicolumn{4}{c}{P 4}& \multirow{2}{*}{Avg.}\\
   & S 1&S 1   &S 2     &S 3     &S 4    &S 1     &S 2     &S 3     &S 4    &S 1     &S 2     &S 3     &S 4  \\
\hline  
 Variant 1 &  88.6&  87.2&     87.1&     87.4&    88.8&  88.2&    87.3&     86.4&    86.4&   87.7&    86.5& 86.4& 87.3& 87.3 \\
 Variant 2 &  83.4&    87.6&     87.5&     86.4&    87.1&  84.0&    84.2&     85.5&    86.8&   83.5&    85.6&     85.6& 87.1&85.7\\
 Variant 3 &  88.1&    86.6&     88.4&     88.0&    87.3&  88.3&    87.4&     85.7&    87.5&   86.5&    88.2&     86.6& 87.6 &87.4\\
 Variant 4 &  86.4&    86.7&     88.5&     86.0&    87.2&  85.2&    86.6&     85.8&    87.8&   85.1&    86.7&     85.6& 87.0 &86.5\\
 Variant 5 &  83.4&    85.1&     85.4&     82.5&   87.0 &  85.9&    87.5&     84.5&    86.4&   86.5&    87.3&     84.5& 86.5&85.6\\
 Variant 6 &  90.2&    86.5&     89.7&     88.9&   89.0 &  87.5&    89.3&     87.4&    89.1&   88.7&    89.1&     87.5 & 89.3&88.6\\
 Variant 7 &  89.8&    89.1&     89.1&    88.3&  88.0 &  89.1&    89.1&     88.8&    88.1&   87.9&    87.9&     85.9&  87.6& 88.4\\
\hline  
Ours & \textbf{91.5}&    \textbf{90.5}&  \textbf{90.3}&     \textbf{89.6}&    \textbf{89.8}&  \textbf{87.6}&    \textbf{89.5}&     \textbf{87.4}&    \textbf{89.7}&   \textbf{87.8}&    \textbf{89.4}&     \textbf{87.8}& \textbf{90.1}& \textbf{89.3}\\
\hline
\end{tabular}

\label{analy}
\end{table*}
