# Supplementary material for: Delving into the Continuous Domain Adaptation
Source: arXiv:2208.13121 source file (2022-08-28)
Supplement: Supplementary file 4 [file complex.tex]

\begin{table*}[!t]
\centering
\small

\setlength\tabcolsep{0.55pt}
%\resizebox{0.85\linewidth}{!}{
\begin{tabular}{c|c|c|c|c|c|c}
\toprule
 Method &Backbone& Params(M) &FLOPs(M) &Backbone& Params(M) &FLOPs(M)\\
 \midrule
 DRT& \multirow{2}{*}{4-layer CNN}&1.86& 0.23& \multirow{2}{*}{ResNet-50} &29.5& 6.45\\
Ours & &1.59&0.048& &23.5& 5.38\\
\bottomrule
\end{tabular}
%}
\caption{Complexity analysis.}
\label{complexity}
\end{table*}
