# Supplementary material for: Delving into the Continuous Domain Adaptation
Source: arXiv:2208.13121 source file (2022-08-28)
Supplement: Supplementary file 6 [file digitda.tex]

\begin{table}[h]
\centering
\caption{Multi-target DA results (\%) in Digit-Five.}
\small
\begin{tabular}{c|c|c|c|c}
\hline
%'mnist', 'usps',  'syn', 'mnist_m', 'svhn'
%mt, up, sv, sy, mm are abbreviations for MNIST, USPS, SVHN, Synthetic Digits, MNIST-M
Dataset &mt & mm & sv& up \\
& $\rightarrow$up, sy& $\rightarrow$mt,up& $\rightarrow$mt,mm&$\rightarrow$sy,mm\\
\hline
SO & 30.9 &92.0 &51.3 &23.0\\
Ours &34.9 &93.4 &73.0 &41.9\\
\hline
\end{tabular}

\label{mtda}
\end{table}
