# Supplementary material for: Delving into the Continuous Domain Adaptation
Source: arXiv:2208.13121 source file (2022-08-28)
Supplement: Supplementary file 8 [file supp_norb.tex]

\begin{table*}[t]
\small
\caption{Comparision Results (\%) in SmallNorb Dataset.}
\centering
% \resizebox{\linewidth}{!}{
\begin{tabular}{c|c|cccc|cccc|cccc|c}
\hline
\multirow{2}{*}{Method}&  P 1& \multicolumn{4}{c|}{P 2} & \multicolumn{4}{c|}{P 3} & \multicolumn{4}{c|}{P 4}& \multirow{2}{*}{Avg.}\\
   & S 1&S 1   &S 2     &S 3     &S 4    &S 1     &S 2     &S 3     &S 4    &S 1     &S 2     &S 3     &S 4  \\
\hline
So &85.1 &88.8 &88.8 &88.8 &88.8 & 86.8 &86.8 &86.8 &86.8 &86.5&86.5&86.5&86.5&87.1\\
So + MMD &78.2 &80.6&82.5 &79.4 &77.4 &80.2 &80.3 &73.8 &72.8 &80.7 &80.1 &78.5&77.0&78.6\\
So + MixStyle &84.0&88.0&88.0&88.0&88.0 &87.1 &87.1 &87.1 &87.1 &87.1 &87.1 &87.1 &87.1&87.1\\
CUA &84.8 & 86.8 &86.4 &83.9 &85.8 &85.5 &87.5 &84.8 &87.4 &82.8 &83.0 &81.0 &85.9 &85.0\\
EDA &45.3 &41.7 &49.0 &65.9 &66.0 &38.1  &42.1 &55.3 &51.8 &39.6 &43.4 &69.9 &65.1 &51.6\\
\hline  
Ours & \textbf{91.5}& \textbf{90.5}& \textbf{ 90.3}&     \textbf{89.6}&    \textbf{89.8}&  \textbf{87.6}&    \textbf{89.5}&     \textbf{87.4}&    \textbf{89.7}&   \textbf{87.8} &    \textbf{89.4}&     \textbf{87.8} &\textbf{90.1} & \textbf{89.3}\\
\hline 
\end{tabular}
% }

\label{sonorb}
\end{table*}
