# Supplementary material for: Delving into the Continuous Domain Adaptation
Source: arXiv:2208.13121 source file (2022-08-28)
Supplement: Supplementary file 9 [file table_digit.tex]

\begin{table}[t]
\centering
\caption{Comparision Results (\%) in five digits datasets.mm and sv are source domains and we test on mm.}
\begin{tabular}{c|c|c}
\hline
\multirow{2}{*}{Method} &\multicolumn{2}{c}{probe target domain}\\
&up & sy \\
\hline
SO &45.4 &45.4\\
CIDA &43.9 &48.6 \\
ATDOC &40.6 &50.1  \\
BCDM &27.6 &40.2\\
\hline 
Ours &\textbf{49.5} &\textbf{53.3}\\
\hline 
\end{tabular}

\label{ana_digits}
\end{table}

% \begin{table*}[t]
% \small
% \caption{Comparision Results (\%) in five digits datasets.\chensays{@yinsong, please change this in priority.}}
% \centering
% \begin{tabular}{c|c|c|c|c}
% \hline 
% Src. Domain& \multicolumn{2}{c|}{up} & \multicolumn{2}{c|}{sy} \\
% \hline 
% mt, sv& mt& up& sy& mm&  sv&  mt& up& sy& mm&  sv&  mt& up& sy& mm&  sv  \\
% \hline  
% SO &99.2&96.7&86.5&45.4&90.3 &99.2&96.1&89.5&45.4&90.3&99.2&96.1&86.5&45.4&90.3\\
% CIDA &93.8&80.6&70.1&43.9&71.5&98.2&92.5&78.9&48.6&84.8 &98.8&93.7&85.9&53.6&88.8\\
% ATDOC &98.3&95.4&73.1&40.6&80.7 &98.9&92.7&83.4&50.1&86.9  &98.1&92.7&75.6&45.2&82.3\\
% BCDM &91.3&25.2&48.5&27.6&68.2 &96.1&88.2&88.3&40.2&82.0&97.4&90.8&89.1&40.7&83.1\\
% DRT &99.1&96.1&83.9&47.7&88.9 &98.7&93.2&79.8&47.19&85.6 &99.1&95.6&84.3&48.9&88.9\\
% \hline  
% Ours &96.2&92.5&72.9&49.5&72.7 &94.3&83.5&76.4&53.3&73.5&89.3&80.6&71.1&55.9&69.6\\
% \hline 
% \end{tabular}
% \label{ana_digits}
% \end{table*}
